# Supplementary material for: Context-aware learning for generative models
Source: arXiv:1507.08272 source file (2020-08-14)
Supplement: Supplementary file 1 [file appendixD.tex]

The results of Figure~\ref{fig:kl_easy} in Section~\ref{subsec:kl} suggest that
the estimation of mixing coefficients with context--aware methods will tend to
be biased. This negative effect is justified and its properties analyzed below.

From Equations~\ref{eq:pzx_c_ca}--\ref{eq:pzx_ca} and
definitions~\ref{eq:p_ca_lat}--\ref{eq:p_wca_obs} in Appendix~\ref{app:proofs},
and given that the marginal distribution $p^{\prime}(z)$ for all cases can be
computed as: 
\begin{equation} 
  p^{\prime}(z)= \int \limits_X p(\bs{x},z)\mathrm{d}\bs{x}
  \label{eq:marg} 
\end{equation} 
replacing the respective joint distribution $p(\bs{x},z)$ for each method in
Equation~\ref{eq:marg} (where $\int \limits_X p(\bs{x}|z)\mathrm{d}\bs{x} =1$
holds for all methods) results in $p^{\prime}(z_i=j)=p_{ij}$ for method
\emph{CA} (for both observed and latent $c$) and $p^{\prime}(z_i=j)=p(z_i=j|c)$
for method \emph{WCA}. Given the above, the mixing coefficients $\hat{\pi}_j$
for method \emph{CA} can be estimated as the average probabilistic label for
mixture $j$: $\hat{\pi}_j=\bar{p}_{j}=\frac{1}{N}\sum_{i=1}^Np_{ij}$, while for
method \emph{WCA} it holds:
$\hat{\pi}_j=\frac{1}{N}\sum_{i=1}^Np(z_i=j|c_i)=\frac{\pi_j}{N}\sum_{i=1}^N
\tilde{p}_{ij} \propto \pi_j\bar{p}_j$, where the tilde denotes the label
weights of the \emph{WCA} case before the normalization (imposed for uniformity
with the other methods, so that the weights become probabilistic labels).

In any case, the average context $\bar{p}_j$ implicitly or explicitly influences
the estimation of mixing coefficients. In the ideal case of ``correct" context,
where the re--distribution of confidence always happens in favour of the correct
class/mixture proportionally to the contextual negentropy, it is still  not
guaranteed that the average probabilistic label is a good estimator of $\pi_j$,
where in general $\pi_j \neq \bar{p}_j$, since $\bar{p}_j=\pi_jc+(1-\pi_j)(1-c)$
and $c \geq 1/M$ the probabilistic label of the correct class for some $NE$.
Figure~\ref{fig:picon}a illustrates the difference $\pi_1 - \bar{p}_1$ for
$\pi_1 \in [0.1, 0.9]$ and $NE \in [0, 1]$ in a two--mixture problem,
where it is shown that the estimation bias will be proportional to the the
deviation of $\pi_j$ from its value when data are uniformly distributed across
mixtures, and inverse proportional to the contextual negentropy $NE$. The
mixture coefficient estimation is thus bound to be biased at low $NE$ for
\emph{CA} and to a certain extent also for \emph{WCA}.

\begin{figure}[h!]
  \centering
  \includegraphics[width=\textwidth]{img/Figure10.pdf}
  \caption{(a) Difference $\pi_1-\bar{p}_1$ and estimation bias
  $\pi_1-\hat{\pi}_1$ for methods (b) \emph{CA} and (c) \emph{WCA}. See text for
details.}
  \label{fig:picon}
\end{figure}

Figure~\ref{fig:picon} investigates experimentally this effect by letting
methods \emph{CA} and \emph{WCA} estimate only the mixing coefficient $\pi_1$ in
the same two--mixture of univariate Gaussians problem, for different $\pi_1 \in
[0.1, 0.9]$ and $NE \in [0, 1]$, where $\hat{\pi}_1^0=\pi_1$ and where method
\emph{US} is able to estimate $\pi_1$ with almost zero bias in all occasions.
Figures~\ref{fig:picon}b and \ref{fig:picon}c verify that the estimation of the
mixing coefficient with context--aware methods tends to be biased following the
same trend of the average probabilistic label $\bar{p}_1$. For method \emph{CA}
this bias is fully determined by the bias of $\bar{p}_1$, as theoretically
predicted, while for method \emph{WCA} the bias is attenuated and its sign
reversed.

While biased estimation of mixing coefficients is certainly a negative property
of context--aware methods, it is positive that its effect is diminished for
balanced problems and with increasing contextual assistance, as well as that it
does not affect the estimation fitness of the internal mixture parameters,
Furthermore, the regular \emph{US} method will be superior in this aspect only
for easy estimation problems. In most situations, \emph{US} will still be
inferior to context--aware methods in the estimation of the mixing coefficients
as a result of getting stack in local maxima of the overall parameter space,
which context--aware methods are largely able to avoid.
